# Supplementary material for: Deep Image Compression using Decoder Side Information
Source: arXiv:2001.04753 source file (2020-07-29)
Supplement: Supplementary file 1 [file fig_L2_vs_si.tex]

\begin{figure}[htb!]
\begin{center}
\begin{tabular}{c}

$Y_{syn}$ using $L_2$ \\
\includegraphics[width=0.95\linewidth]{Images/supplementary/correlation/2900_bpp007_si_L2_vs_si.png}\\

$Y_{syn}$ using Pearson + mask \\
\includegraphics[width=0.95\linewidth]{Images/supplementary/correlation/2900_bpp007_si_vs_L2.png}\\

\end{tabular}
\end{center}

  \caption{$Y_{syn}$ when similarity measure between patches is taken to be $L_2$. Patch choice based on color has improved, but wrong structure-based choices are seen.} 
\label{fig:L2}

\end{figure}
